# Supplementary material for: Metric Learning for Image Registration
Source: arXiv:1904.09524 source file (2019-04-21)
Supplement: Supplementary file 1 [file supplementary_material.tex]

\section{Generating the synthetic test cases}

\begin{figure}
  \begin{tabular}{llll}
    (a) & 
    \includegraphics[height=0.225\textheight]{figs/example_synthetic_case_generation/cropped-circle_init_m_smoothed_orig_0.pdf} &
    (b) & \includegraphics[height=0.225\textheight]{figs/example_synthetic_case_generation/cropped-random_source_m_smoothed_orig_0.pdf} \\
    (c) & \includegraphics[height=0.225\textheight]{figs/example_synthetic_case_generation/cropped-source_image_0.pdf} &
    (d) & \includegraphics[height=0.225\textheight]{figs/example_synthetic_case_generation/cropped-target_image_with_grid_0.pdf} \\
    (e) & \includegraphics[height=0.225\textheight]{figs/example_synthetic_case_generation/cropped-std_im_orig_0.pdf} &
    (f) & \includegraphics[height=0.225\textheight]{figs/example_synthetic_case_generation/cropped-std_im_source_0.pdf}
  \end{tabular}
  \caption{Illustration of the intermediate steps during synthetic test case generation, as described in Sect.~\ref{subsec:synthetic_experiment_setup}. %This example shows the generation of one \emph{source} image.} 
  (a) A shape with concentric circles and a smoothed momentum field (based on a random unsmoothed momentum field on the edges of the shape) is generated (randomly); (b) the momentum from (a) results in a deformed shape. This shape is considered the \emph{source} image. Again, a random smoothed momentum field is generated; (c) Random noise is added to the source image and it is deformed based on the momentum in (b) to result in the textured target image (d). Each ring has a different multi-Gaussian weight. The resulting standard deviations of the original concentric shape of (a) and of the generated source image in (c) are shown in (e) and (f), respectively.}
  \label{fig:example_generation}
\end{figure}
